# Supplementary material for: Task-Guided Inverse Reinforcement Learning Under Partial Information
Source: arXiv:2105.14073 source file (2021-12-16)
Supplement: Supplementary file 1 [file avoid_mem1_trajsize10mdp_irl_si.tex]

% $\mathrm{Guided \ policy, \ |n|=1}$
x	y	err
0	0.0	0.0
1	0.0	0.0
2	-0.09999999999999991	9.71445146547012e-17
3	-0.09999999999999991	9.71445146547012e-17
4	-0.19999999999999982	1.942890293094024e-16
5	-0.19999999999999982	1.942890293094024e-16
6	-0.29999999999998495	1.509903313490213e-14
7	-0.29999999999998495	1.509903313490213e-14
8	-0.39999999999999963	3.885780586188048e-16
9	-0.39999999999999963	3.885780586188048e-16
10	-0.5	0.0
11	-0.5	0.0
12	-0.5999999999999699	3.008704396734174e-14
13	-0.5999999999999699	3.008704396734174e-14
14	-0.7000000000000268	2.6867397195928788e-14
15	-0.7000000000000268	2.6867397195928788e-14
16	-0.7999999999999993	6.661338147750939e-16
17	-0.7999999999999993	6.661338147750939e-16
18	-0.9000000000000503	5.040412531798211e-14
19	-0.9000000000000503	5.040412531798211e-14
20	-0.9995666666666669	0.006568527655080217
21	4.350433333333334	15.455513788900607
22	4.261566666666483	15.486279288848644
23	4.261566666666483	15.486279288848644
24	4.172699999999827	15.51704755132255
25	4.172699999999827	15.51704755132255
26	4.083833333333504	15.547818559921241
27	4.083833333333504	15.547818559921241
28	3.9949666666668464	15.57859229837221
29	3.9949666666668464	15.57859229837221
30	3.906100000000001	15.609368750528954
31	3.906100000000001	15.609368750528954
32	3.817299999999839	15.640125022198205
33	7.167300000000147	19.094373535416068
34	7.0851999999997	19.132071528195574
35	7.0851999999997	19.132071528195574
36	7.003100000000316	19.169772048461986
37	7.269766666667006	19.39194152078513
38	7.188199999999873	19.43009214491809
39	7.188199999999873	19.43009214491809
40	7.106633333333347	19.46824523847852
41	7.106633333333347	19.46824523847852
42	7.025066666666791	19.5064007869781
43	7.025066666666791	19.5064007869781
44	6.943533333333043	19.544543266998158
45	8.54353333333301	20.740536754116707
46	8.465200000000342	20.78111439809398
47	8.465200000000342	20.78111439809398
48	8.38699999999974	20.82162572102989
49	9.30366666666634	21.41861308664899
50	9.227300000000005	21.46034322597554
51	9.227300000000005	21.46034322597554
52	9.150933333333668	21.502076313593008
53	9.150933333333668	21.502076313593008
54	9.074566666666321	21.543812332366063
55	9.074566666666321	21.543812332366063
56	8.998233333333689	21.585533123187293
57	9.814900000000364	22.064251206948697
58	9.740199999999646	22.106961285833055
59	9.740199999999646	22.106961285833055
60	9.665533333333347	22.1496553483089
61	10.748866666666682	22.719117472198835
62	10.676366666667057	22.762993610951888
63	10.676366666667057	22.762993610951888
64	10.603866666666327	22.806872759080864
65	10.653866666666328	22.831350340753442
66	10.581466666667026	22.875283528637457
67	10.581466666667026	22.875283528637457
68	10.509066666666305	22.919219688481686
69	10.859066666666289	23.085315342490837
70	10.787366666666676	23.12960362246203
71	10.787366666666676	23.12960362246203
72	10.715733333333715	23.173853782417353
73	11.832400000000439	23.65675555889522
74	11.762999999999847	23.702029962291093
75	11.762999999999847	23.702029962291093
76	11.69363333333356	23.747285798567813
77	11.793633333333553	23.787073299004543
78	11.7244666666663	23.83241716756554
79	11.7244666666663	23.83241716756554
80	11.655300000000034	23.877764242980163
81	11.755300000000037	23.91665873911623
82	11.68633333333377	23.962092699836163
83	11.68633333333377	23.962092699836163
84	11.617433333333164	24.00748604245981
85	12.617433333333388	24.36646300578396
86	12.550533333333409	24.412638251164182
87	12.550533333333409	24.412638251164182
88	12.483666666666291	24.458793917299214
89	12.766999999999625	24.55099952479917
90	12.700700000000047	24.597360756322743
91	12.700700000000047	24.597360756322743
92	12.634400000000465	24.643725434817867
93	12.717733333333806	24.669830269559505
94	12.65160000000007	24.716256272070925
95	12.65160000000007	24.716256272070925
96	12.58546666666672	24.76268568058749
97	13.218799999999984	24.94863857127236
98	13.153933333332956	24.99548928364702
99	13.153933333332956	24.99548928364702
100	13.089100000000043	25.042319338604976
101	13.489100000000045	25.149283843813112
102	13.42506666666714	25.196361212065806
103	13.42506666666714	25.196361212065806
104	13.361033333333447	25.24344201831907
105	13.561033333333476	25.293614838509498
106	13.497399999999955	25.34081529680237
107	13.497399999999955	25.34081529680237
108	13.433799999999618	25.38799449004763
109	14.00046666666627	25.51896379392291
110	13.93800000000004	25.566455027373248
111	13.93800000000004	25.566455027373248
112	13.8755333333338	25.613949741932164
113	14.408866666667159	25.723194618519045
114	14.34746666666689	25.770956525687417
115	14.34746666666689	25.770956525687417
116	14.286066666666548	25.818721873779698
117	14.386066666666547	25.837553790214017
118	14.324866666666278	25.88536912972655
119	14.324866666666278	25.88536912972655
120	14.263700000000048	25.933161890586234
121	14.41370000000005	25.960109314934588
122	14.352833333333821	26.00797349478699
123	14.352833333333821	26.00797349478699
124	14.291966666666887	26.055841164677737
125	15.091966666666995	26.181667481889743
126	15.032699999999801	26.229867213604166
127	15.032699999999801	26.229867213604166
128	14.973433333332954	26.27807040503953
129	15.356766666666276	26.328129586918795
130	15.298266666666725	26.37647393029568
131	15.298266666666725	26.37647393029568
132	15.239766666667173	26.42482170130068
133	15.506433333333842	26.455350094305086
134	15.448466666667024	26.50378949601162
135	15.448466666667024	26.50378949601162
136	15.390533333333103	26.552204498224693
137	15.823866666666405	26.59448546313459
138	15.766799999999613	26.64303369413259
139	15.766799999999613	26.64303369413259
140	15.709733333333386	26.691585414299745
141	15.976400000000057	26.713125919167545
142	15.919866666667163	26.761752906879654
143	15.919866666667163	26.761752906879654
144	15.86333333333369	26.810383353386456
145	16.13000000000039	26.828314023310373
146	16.073999999999742	26.877013549376038
147	16.073999999999742	26.877013549376038
148	16.01799999999962	26.925716505476913
149	16.534666666666265	26.951103840515103
150	16.479700000000058	26.99992020809211
151	16.479700000000058	26.99992020809211
152	16.424733333333847	27.04873998782398
153	16.64140000000052	27.055683433245754
154	16.586866666667067	27.104546005830574
155	16.586866666667067	27.104546005830574
156	16.532333333333057	27.153411962813028
157	16.765666666666363	27.15814637554554
158	16.711599999999592	27.207053597183013
159	16.711599999999592	27.207053597183013
160	16.65753333333339	27.255964177568636
161	17.024200000000054	27.258104868583267
162	16.970866666667185	27.30706900997526
163	16.970866666667185	27.30706900997526
164	16.917533333333747	27.356036492559216
165	17.417533333333765	27.349318076487663
166	17.36519999999972	27.39833928592459
167	17.36519999999972	27.39833928592459
168	17.312866666666284	27.447363828162782
169	17.47953333333295	27.442528693900908
170	17.427533333333404	27.491568681729206
171	17.427533333333404	27.491568681729206
172	17.375533333333852	27.54061197665917
173	17.74220000000053	27.525178882131012
174	17.690933333333792	27.574243860208245
175	17.690933333333792	27.574243860208245
176	17.639666666666365	27.623312133453854
177	17.939666666666366	27.60604233174702
178	17.888999999999623	27.65512054454508
179	17.888999999999623	27.65512054454508
180	17.838333333333402	27.704202037877508
181	18.205000000000073	27.677432232777402
182	18.15506666666718	27.726514884893678
183	18.15506666666718	27.726514884893678
184	18.10513333333378	27.77560080926349
185	18.305133333333778	27.758277089585274
186	18.25559999999971	27.807360332113586
187	18.25559999999971	27.807360332113586
188	18.206066666666306	27.85644682765966
189	18.606066666666297	27.816124398070105
190	18.557333333333403	27.865192138021733
191	18.557333333333403	27.865192138021733
192	18.508600000000513	27.914263129088713
193	18.741933333333854	27.8872903236503
194	18.69366666666712	27.936345499884265
195	18.69366666666712	27.936345499884265
196	18.645399999999704	27.985403912992336
197	18.8453999999997	27.960054938668183
198	18.79753333333297	28.009096508972064
199	18.79753333333297	28.009096508972064
200	18.74966666666674	28.058141300204273
201	18.98300000000008	28.025970176487043
202	18.935600000000516	28.07499040023591
203	18.935600000000516	28.07499040023591
204	18.888233333333805	28.123979416367323
205	19.088233333333804	28.094179555183235
206	19.041266666666377	28.143144050766935
207	19.041266666666377	28.143144050766935
208	18.994299999999665	28.192111854973575
209	19.227633333332996	28.15475187362762
210	19.18113333333342	28.203686119292563
211	19.18113333333342	28.203686119292563
212	19.134633333333838	28.252623663396893
213	19.38463333333384	28.209589277387263
214	19.33863333333381	28.25848540643232
215	19.33863333333381	28.25848540643232
216	19.29263333333304	28.307384826794355
217	19.759299999999687	28.219446017064037
218	19.714233333333006	28.26825110871846
219	19.714233333333006	28.26825110871846
220	19.66916666666675	28.317059510223764
221	19.91916666666675	28.265858840166842
222	19.87460000000049	28.314610624905036
223	19.87460000000049	28.314610624905036
224	19.830033333333812	28.36336571469544
225	20.030033333333822	28.320107721056353
226	19.985866666666357	28.36881422000022
227	19.985866666666357	28.36881422000022
228	19.94169999999968	28.41752401441756
229	20.175033333333015	28.364445467266552
230	20.13133333333342	28.413093546618526
231	20.13133333333342	28.413093546618526
232	20.087700000000492	28.46167081140264
233	20.337700000000495	28.401766765056507
234	20.294566666667162	28.450271829027592
235	20.294566666667162	28.450271829027592
236	20.251433333333022	28.49878040569875
237	20.418099999999686	28.45702424809539
238	20.375299999999694	28.505482745897996
239	20.375299999999694	28.505482745897996
240	20.332500000000092	28.55394474353211
241	20.582500000000095	28.488576840843944
242	20.540200000000493	28.536957276953764
243	20.540200000000493	28.536957276953764
244	20.49793333333383	28.58530314215516
245	20.88126666666718	28.479305862249273
246	20.839766666666353	28.52751365399534
247	20.839766666666353	28.52751365399534
248	20.798266666666382	28.575725076753773
249	20.998266666666385	28.51758680175388
250	20.957166666666765	28.565722733821488
251	20.957166666666765	28.565722733821488
252	20.916100000000483	28.613823304887635
253	21.049433333333816	28.57380174820201
254	21.008633333333847	28.621851013963976
255	21.008633333333847	28.621851013963976
256	20.967899999999695	28.669825593993746
257	21.084566666666362	28.63388630880504
258	21.044066666666392	28.681814879738038
259	21.044066666666392	28.681814879738038
260	21.00356666666677	28.729747370026885
261	21.2369000000001	28.655580173094716
262	21.196866666667148	28.703412866455388
263	21.196866666667148	28.703412866455388
264	21.156833333333843	28.751249479611847
265	21.373500000000522	28.679832189478624
266	21.333899999999705	28.727571903254344
267	21.333899999999705	28.727571903254344
268	21.294299999999737	28.77531553565785
269	21.52763333333306	28.695650072189444
270	21.4885000000001	28.74328416198555
271	21.4885000000001	28.74328416198555
272	21.449366666667142	28.790922173471493
273	21.566033333333813	28.749934543674353
274	21.527133333333847	28.797517782768995
275	21.527133333333847	28.797517782768995
276	21.488266666666366	28.845064205086558
277	21.62159999999969	28.797159815509797
278	21.582999999999736	28.844641287421283
279	21.582999999999736	28.844641287421283
280	21.544400000000106	28.892126758686413
281	21.744400000000105	28.818348818764623
282	21.70620000000047	28.8657316131081
283	21.70620000000047	28.8657316131081
284	21.66800000000051	28.91311840670271
285	21.734666666667177	28.887971629882454
286	21.6965999999997	28.935325960493717
287	21.6965999999997	28.935325960493717
288	21.65853333333308	28.9826842646126
289	21.958533333333083	28.866431493730172
290	21.92106666666677	28.913624404345423
291	21.92106666666677	28.913624404345423
292	21.883600000000463	28.960821311558423
293	22.083600000000438	28.880715556232374
294	22.046533333333848	28.92779876374212
295	22.046533333333848	28.92779876374212
296	22.009499999999704	28.974843682350933
297	22.159499999999703	28.913253300461925
298	22.122766666666468	28.96021118153129
299	22.122766666666468	28.96021118153129
