# Supplementary material for: Task-Guided Inverse Reinforcement Learning Under Partial Information
Source: arXiv:2105.14073 source file (2021-12-16)
Supplement: Supplementary file 3 [file evade_mem1_trajsize10mdp_irl_si.tex]

% $\mathrm{Guided \ policy, \ |n|=1}$
x	y	err
0	0.0	0.0
1	0.0	0.0
2	-0.09999999999999991	9.71445146547012e-17
3	-0.09999999999999991	9.71445146547012e-17
4	-0.19999999999999982	1.942890293094024e-16
5	-0.19999999999999982	1.942890293094024e-16
6	-0.29999999999998495	1.509903313490213e-14
7	-0.29999999999998495	1.509903313490213e-14
8	-0.3999666666666663	0.0018254375426790712
9	-0.40019999999999967	0.005160103358138066
10	-0.49983333333333335	0.004827582785986618
11	-0.5001666666666665	0.007525881269916949
12	-0.5996999999999699	0.008361220006673371
13	-0.6474666666666651	0.05092722476458099
14	-0.6998000000000267	0.012908395201056628
15	-0.7508333333333325	0.05182636609123055
16	-0.7995666666666662	0.016826929474968114
17	-0.09170000000000197	3.851987509931294
18	3.8822333333335233	8.541723928978842
19	6.367633333333363	9.657972651246446
20	7.105966666666651	9.866235742785745
21	7.933066666666679	10.015866409297143
22	8.877100000000034	10.09404934883262
23	9.495166666666558	10.096791238089262
24	10.003566666666426	10.074317376984771
25	10.482833333333247	10.025574728607316
26	11.068233333333284	9.92605531982478
27	11.643899999999764	9.787339924105911
28	11.958933333333007	9.702726431037613
29	12.28963333333309	9.597770359075838
30	12.739866666666519	9.425973547361258
31	13.052799999999902	9.293039267465993
32	13.357933333333254	9.15014555779793
33	13.645799999999866	9.000450860558885
34	13.90553333333314	8.856391066092105
35	14.17523333333308	8.690230718775814
36	14.41649999999968	8.533310284799509
37	14.68073333333299	8.343721519535286
38	14.890366666666335	8.186462231364368
39	15.142233333333053	7.97960815739438
40	15.340466666666451	7.8082863537540845
41	15.51303333333314	7.651230410782851
42	15.719033333333137	7.4503611365862845
43	15.925933333333118	7.234316424437682
44	16.072866666666403	7.074796377438887
45	16.22746666666634	6.896751330558196
46	16.34829999999965	6.753181258488458
47	16.470299999999664	6.59989302261789
48	16.578466666666362	6.460214365552412
49	16.661099999999717	6.349054269994365
50	16.74979999999974	6.226060816707008
51	16.845999999999744	6.084925965038502
52	16.93563333333308	5.949280651100189
53	17.018633333333074	5.819468715632194
54	17.082266666666374	5.716960048448417
55	17.11876666666635	5.659706512905194
56	17.18943333333301	5.538266125683177
57	17.233033333333022	5.4639508415513225
58	17.290399999999707	5.360521228388156
59	17.37459999999972	5.200571908293685
60	17.45229999999972	5.046779967794643
61	17.503499999999722	4.9426299763722366
62	17.554866666666396	4.833758680594477
63	17.62636666666639	4.675783157100264
64	17.66479999999972	4.588628803175607
65	17.709899999999713	4.482990667326159
66	17.761733333333037	4.356231819155408
67	17.78059999999971	4.310216194113627
68	17.812499999999712	4.229327813021768
69	17.851466666666383	4.125302960457013
70	17.856899999999712	4.113346454733244
71	17.862533333333047	4.099827994223952
72	17.89469999999972	4.01152613228431
73	17.90709999999971	3.9780321253101762
74	17.932699999999706	3.9052982015889164
75	17.94523333333304	3.869522444120885
76	17.957633333333042	3.8341441981519155
77	17.97016666666638	3.79711205684299
78	17.98936666666638	3.738550110968494
79	18.008699999999713	3.67725816925233
80	18.03473333333304	3.59218600050475
81	18.040799999999713	3.573321800976418
82	18.053533333333046	3.53092540026294
83	18.05963333333304	3.5111243022080183
84	18.065799999999708	3.4907807665334394
85	18.078599999999707	3.4464796590144404
86	18.07813333333304	3.449529704499167
87	18.084233333333042	3.4284673075426952
88	18.08379999999971	3.4313259186501024
89	18.083266666666375	3.434845944467161
90	18.08949999999971	3.413217409327024
91	18.08899999999971	3.4165507460010174
92	18.08859999999971	3.4192245768107288
93	18.101499999999707	3.3717029945316193
94	18.101066666666373	3.3746524061334586
95	18.107266666666373	3.351866225784601
96	18.113599999999707	3.3281999699537086
97	18.126499999999705	3.278679777491722
98	18.12623333333304	3.2805662842800887
99	18.139199999999708	3.2289724929147665
100	18.138866666666374	3.231377835468279
101	18.158633333333047	3.149826259582512
102	18.15833333333304	3.1520581459667736
103	18.158099999999706	3.153792593582105
104	18.157799999999707	3.1560311299689867
105	18.15753333333304	3.1580199359022014
106	18.17733333333304	3.071999276620289
107	18.183733333333038	3.044021801644799
108	18.196899999999705	2.9852270248675756
109	18.196699999999705	2.986823135596254
110	18.19656666666637	2.9878897032669696
111	18.19636666666637	2.9894910601787887
112	18.2028999999997	2.959188220328897
113	18.216099999999702	2.8967149422521317
114	18.215999999999703	2.8975479288529455
115	18.222533333333036	2.866237763263149
116	18.22243333333304	2.867083316814418
117	18.222333333333037	2.867932104418685
118	18.222199999999702	2.869063812465685
119	18.222133333333037	2.8696324007711493
120	18.22866666666637	2.836835952645525
