# Supplementary material for: Task-Guided Inverse Reinforcement Learning Under Partial Information
Source: arXiv:2105.14073 source file (2021-12-16)
Supplement: Supplementary file 7 [file maze_mem10_trajsize5mdp_irl_si.tex]

% $\mathrm{Guided \ policy, \ |n|=10}$
x	y	err
0	0.0	0.0
1	-0.09999999999999647	3.5388358909926865e-15
2	0.17000000000000764	5.537427200424331
3	0.15709999999999658	6.255978707604308
4	0.07979999999999682	6.514345090644052
5	3.4276500000000016	14.146402739830924
6	8.02739999999977	19.417430809455478
7	14.11664999999965	23.29158512805641
8	20.413249999999998	25.17700477494287
9	25.827599999999602	25.44806531428251
10	30.527900000000027	24.688057874000588
11	34.237750000000354	23.46813094256753
12	37.15045000000049	21.99933066703396
13	39.24914999999983	20.623262575972188
14	40.92720000000017	19.26859621664223
15	42.14875000000007	18.122730987284946
16	42.91785000000001	17.334919854948904
17	43.82360000000023	16.212893111348183
18	44.52624999999999	15.257771984713273
19	45.14535000000014	14.23835483395113
20	45.53070000000012	13.637810216820014
21	46.00190000000007	12.65595853303893
22	46.27405000000012	12.08911252315481
23	46.39675000000007	11.768274488534864
24	46.694700000000104	10.947708523248162
25	46.89325000000008	10.382463071810017
26	46.917200000000086	10.328946420618049
27	47.01620000000009	9.96825097798001
28	47.09040000000009	9.73271379626463
29	47.18975000000009	9.422775065632257
30	47.26430000000009	9.113385513079074
31	47.26400000000009	9.115041634573059
32	47.26370000000009	9.116700736011955
33	47.26340000000009	9.118362815769093
34	47.288100000000085	9.049371712445033
35	47.33785000000009	8.907031625491184
36	47.357700000000094	8.86637303016293
37	47.35765000000009	8.866660672288127
38	47.38260000000009	8.7928537597301
39	47.38260000000009	8.7928537597301
40	47.38260000000009	8.7928537597301
41	47.38260000000009	8.7928537597301
42	47.38260000000009	8.7928537597301
43	47.38260000000009	8.7928537597301
44	47.38260000000009	8.7928537597301
45	47.38260000000009	8.7928537597301
46	47.38260000000009	8.7928537597301
47	47.38260000000009	8.7928537597301
48	47.38260000000009	8.7928537597301
49	47.38260000000009	8.7928537597301
50	47.38260000000009	8.7928537597301
51	47.38260000000009	8.7928537597301
52	47.38260000000009	8.7928537597301
53	47.38260000000009	8.7928537597301
54	47.38260000000009	8.7928537597301
55	47.38260000000009	8.7928537597301
56	47.38260000000009	8.7928537597301
57	47.38260000000009	8.7928537597301
58	47.38260000000009	8.7928537597301
59	47.38260000000009	8.7928537597301
60	47.38260000000009	8.7928537597301
61	47.38260000000009	8.7928537597301
62	47.38260000000009	8.7928537597301
63	47.38260000000009	8.7928537597301
64	47.38260000000009	8.7928537597301
65	47.38260000000009	8.7928537597301
66	47.38260000000009	8.7928537597301
67	47.38260000000009	8.7928537597301
68	47.38260000000009	8.7928537597301
69	47.38260000000009	8.7928537597301
70	47.38260000000009	8.7928537597301
71	47.38260000000009	8.7928537597301
72	47.38260000000009	8.7928537597301
73	47.38260000000009	8.7928537597301
74	47.38260000000009	8.7928537597301
75	47.38260000000009	8.7928537597301
76	47.38260000000009	8.7928537597301
77	47.38260000000009	8.7928537597301
78	47.38260000000009	8.7928537597301
79	47.38260000000009	8.7928537597301
80	47.38260000000009	8.7928537597301
81	47.38260000000009	8.7928537597301
82	47.38260000000009	8.7928537597301
83	47.38260000000009	8.7928537597301
84	47.38260000000009	8.7928537597301
85	47.38260000000009	8.7928537597301
86	47.38260000000009	8.7928537597301
87	47.38260000000009	8.7928537597301
88	47.38260000000009	8.7928537597301
89	47.38260000000009	8.7928537597301
90	47.38260000000009	8.7928537597301
91	47.38260000000009	8.7928537597301
92	47.38260000000009	8.7928537597301
93	47.38260000000009	8.7928537597301
94	47.38260000000009	8.7928537597301
95	47.38260000000009	8.7928537597301
96	47.38260000000009	8.7928537597301
97	47.38260000000009	8.7928537597301
98	47.38260000000009	8.7928537597301
99	47.38260000000009	8.7928537597301
