# Supplementary material for: Task-Guided Inverse Reinforcement Learning Under Partial Information
Source: arXiv:2105.14073 source file (2021-12-16)
Supplement: Supplementary file 8 [file maze_mem10_trajsize5pomdp_irl_si.tex]

% $\mathrm{Guided \ policy, \ |n|=10}$
x	y	err
0	0.0	0.0
1	-0.09999999999999647	3.5388358909926865e-15
2	0.04499999999999918	4.635728098152354
3	0.01655000000000124	5.339939240993198
4	0.34855000000000635	7.13732007811769
5	1.1715999999999998	9.837755508244701
6	2.73164999999998	13.152513572602594
7	5.345099999999955	16.88471042067335
8	7.964050000000215	19.558183008589786
9	11.21344999999989	21.961060404668785
10	14.474599999999976	23.661718129501587
11	17.59745000000037	24.758588782430675
12	20.746750000000034	25.408875210002794
13	23.237499999999844	25.666569575032643
14	25.558549999999606	25.64100011500145
15	28.389350000000004	25.289293220204726
16	30.33090000000036	24.861058810718436
17	32.116500000000414	24.331886234938608
18	33.87089999999976	23.65065523806897
19	35.12889999999988	23.08613533682084
20	36.47465000000003	22.31758818460211
21	37.7281500000001	21.54513129636266
22	38.9993000000003	20.6013504292799
23	39.9030499999999	19.84431318281136
24	40.66365000000004	19.135344618728535
25	41.34580000000004	18.46346750640303
26	41.97935000000003	17.815874342212332
27	42.51920000000019	17.202198445547634
28	43.095149999999975	16.467295511938286
29	43.5623000000001	15.835704553634455
30	43.900400000000054	15.357640112985981
31	44.26920000000003	14.79324107016453
32	44.43875000000014	14.508579649211079
33	44.678650000000005	14.075466925736382
34	44.92405000000007	13.674468421020952
35	45.23995000000004	13.081535422017504
36	45.386550000000014	12.700860762070485
37	45.55845000000007	12.376471573009024
38	45.7307	11.97556334833563
39	45.82330000000005	11.8017666944403
40	45.94610000000004	11.502121316957217
41	45.99415000000002	11.379976308301337
42	46.06730000000007	11.221449135918263
43	46.24060000000001	10.75636609826945
44	46.289250000000045	10.596347457378839
45	46.35800000000002	10.42138215401392
46	46.48190000000001	10.085799541434527
47	46.531050000000036	9.909574708205133
48	46.63030000000001	9.566009194538704
49	46.649750000000026	9.529353070250936
50	46.67425000000002	9.40920198196957
51	46.673800000000014	9.411887885010158
52	46.673350000000035	9.414577780097243
53	46.66790000000002	9.452762008534796
54	46.71745000000003	9.31113744380886
55	46.71210000000002	9.354728408136733
56	46.711750000000016	9.35700416466192
57	46.711400000000026	9.359283094340086
58	46.73605000000002	9.260816670116046
59	46.73575000000003	9.262789911117478
60	46.76045000000002	9.18958599706758
61	46.76020000000002	9.191294574759247
62	46.75995000000003	9.193005547561699
63	46.784700000000015	9.11807248874452
64	46.78450000000002	9.1195120346431
65	46.784300000000016	9.120953541708282
66	46.809100000000015	8.960931714392222
67	46.833950000000016	8.853827556345328
68	46.83385000000001	8.854489210423184
69	46.85875000000002	8.745078812537901
70	46.85870000000002	8.745386458584896
71	46.883650000000024	8.662483343562641
72	46.883650000000024	8.662483343562641
73	46.883650000000024	8.662483343562641
74	46.883650000000024	8.662483343562641
75	46.883650000000024	8.662483343562641
76	46.883650000000024	8.662483343562641
77	46.883650000000024	8.662483343562641
78	46.883650000000024	8.662483343562641
79	46.883650000000024	8.662483343562641
80	46.883650000000024	8.662483343562641
81	46.883650000000024	8.662483343562641
82	46.883650000000024	8.662483343562641
83	46.883650000000024	8.662483343562641
84	46.883650000000024	8.662483343562641
85	46.883650000000024	8.662483343562641
86	46.883650000000024	8.662483343562641
87	46.883650000000024	8.662483343562641
88	46.883650000000024	8.662483343562641
89	46.883650000000024	8.662483343562641
90	46.883650000000024	8.662483343562641
91	46.883650000000024	8.662483343562641
92	46.883650000000024	8.662483343562641
93	46.883650000000024	8.662483343562641
94	46.883650000000024	8.662483343562641
95	46.883650000000024	8.662483343562641
96	46.883650000000024	8.662483343562641
97	46.883650000000024	8.662483343562641
98	46.883650000000024	8.662483343562641
99	46.883650000000024	8.662483343562641
