# Supplementary material for: Task-Guided Inverse Reinforcement Learning Under Partial Information
Source: arXiv:2105.14073 source file (2021-12-16)
Supplement: Supplementary file 9 [file maze_mem1_trajsize5mdp_irl_si.tex]

% $\mathrm{Guided \ policy, \ |n|=1}$
x	y	err
0	0.0	0.0
1	-0.09999999999999647	3.5388358909926865e-15
2	0.7749999999999734	9.555070643380835
3	1.0622500000000206	11.859932543547425
4	1.5385499999999601	13.773174249152072
5	2.3727500000000004	15.989394686401003
6	3.165049999999933	17.65174533856342
7	4.474700000000038	19.69769453286341
8	5.868150000000125	21.588139117985442
9	6.75015000000018	22.834502621636375
10	8.539699999999996	24.465228670707432
11	9.74325000000001	25.563597447102232
12	11.304749999999693	26.596336447667184
13	12.349700000000247	27.412160073770057
14	13.707149999999725	28.13855067123227
15	14.667599999999958	28.673693522809124
16	15.97025000000027	29.189939875537444
17	17.270849999999804	29.617650738664445
18	18.349400000000063	29.936058351760266
19	19.34534999999966	30.19042047367846
20	20.36354999999998	30.421750547881288
21	21.244050000000325	30.587274553276128
22	22.401650000000213	30.611238496302555
23	23.366749999999808	30.67017915561491
24	24.33894999999972	30.67224425922401
25	24.948300000000003	30.61090601583031
26	25.69900000000027	30.553495201040512
27	26.276400000000226	30.517974261736367
28	26.89519999999982	30.31562743800621
29	27.790349999999762	30.151055402381914
30	28.47239999999999	30.000958955340053
31	29.040950000000212	29.777746189016714
32	29.495700000000213	29.590542433520945
33	30.171449999999822	29.070986393610642
34	30.743599999999823	28.806046223666304
35	31.33695	28.33716093220177
36	31.68655000000017	28.03132201836914
37	32.00190000000019	27.795211932813196
38	32.49294999999986	27.548888095484003
39	32.83509999999989	27.191564647699074
40	33.20805000000002	26.88857731821263
41	33.546800000000125	26.62450956844086
42	33.78125000000017	26.43306666729191
43	34.0611999999999	26.310510153929016
44	34.25174999999997	26.10720450254101
45	34.51285000000004	25.834122781265542
46	34.72950000000007	25.629329483035566
47	34.91660000000016	25.334131412779886
48	35.07909999999995	25.234087326273595
49	35.19695000000003	25.134547652533943
50	35.54005000000005	24.82365668062426
51	35.55885000000007	24.821238721657288
52	35.74770000000014	24.70773147640225
53	35.911949999999976	24.462609676759783
54	35.97655000000004	24.397152602250568
55	36.066300000000055	24.315806264855834
56	36.161250000000074	24.21723525585652
57	36.226400000000126	24.007274585841667
58	36.2667	23.98388648884911
59	36.45710000000005	23.7907339018787
60	36.55290000000006	23.652983777739376
61	36.61890000000009	23.63325417266943
62	36.63505000000012	23.652695544007347
63	36.75125000000002	23.544893680743215
64	36.81770000000005	23.452599998933977
65	36.90430000000007	23.40534087574882
66	36.951150000000084	23.373662928122762
67	37.058100000000124	23.220172143849442
68	37.10530000000005	23.1219523810166
69	37.22760000000009	22.982183495917102
70	37.3501500000001	22.630870729547816
71	37.37295000000011	22.61496502976519
72	37.430800000000126	22.588359642966505
73	37.453800000000065	22.571788709803137
74	37.536850000000086	22.490850074585847
75	37.68515000000009	22.271422147620044
76	37.7037500000001	22.270634273354208
77	37.77240000000012	22.092835224117298
78	37.771200000000086	22.09623543864427
79	37.79000000000009	22.08997306471879
80	37.8138500000001	22.047086954459562
81	37.83275000000011	22.04717742563651
82	37.85670000000012	22.015071771629533
83	37.85570000000009	22.018074337007832
84	37.929700000000096	21.902834928611437
85	37.97885000000011	21.82209058906823
86	37.978100000000104	21.82444570636327
87	37.967350000000124	21.86647705913096
88	37.9916000000001	21.80960658608948
89	37.990900000000096	21.811843507370014
90	38.0352000000001	21.789288445472422
91	38.05960000000012	21.65075605700641
92	38.05405000000012	21.671472806376098
93	38.0535000000001	21.673226980539848
94	38.052950000000116	21.6749835362682
95	38.10240000000011	21.601468103811854
96	38.101950000000116	21.602969962426506
97	38.126500000000114	21.54327244756466
98	38.151100000000106	21.4947193233594
99	38.15075000000011	21.4958963394761
