# Supplementary material for: Task-Guided Inverse Reinforcement Learning Under Partial Information
Source: arXiv:2105.14073 source file (2021-12-16)
Supplement: Supplementary file 11 [file obstacle_mem1_trajsize10mdp_irl_si.tex]

% $\mathrm{Guided \ policy, \ |n|=1}$
x	y	err
0	0.0	0.0
1	-5.0	0.0
2	-9.78	1.0254754994635464
3	-13.886666666666667	18.525491146586038
4	-13.61	53.53613639402983
5	-11.768333333333333	78.18235945887027
6	-7.168333333333333	102.83849796593395
7	-3.486666666666667	120.415294525052
8	-0.22833333333333333	134.6819940844151
9	1.43	145.0044428055027
10	5.556666666666667	157.5238292731886
11	8.476666666666667	167.33552956725987
12	10.366666666666667	175.1971714637226
13	11.51	181.79966969167234
14	13.9	189.16106012249114
15	16.02	195.84920117274487
16	16.856666666666666	201.17708481722414
17	18.748333333333335	207.0513020096417
18	21.033333333333335	212.8973905168612
19	23.546666666666667	218.5824508560137
20	26.625	224.2901417992626
21	28.758333333333333	229.19005926062835
22	33.303333333333335	234.99930068453907
23	38.263333333333335	240.57819377953217
24	43.13666666666666	245.71516977092887
25	48.25833333333333	250.55380313196315
26	55.145	255.48940742882814
27	62.29833333333333	259.9790235074525
28	72.245	264.4090927111512
29	82.82333333333334	268.1532126519347
30	89.15666666666667	270.9417627256609
31	97.935	273.3658003024522
32	106.65666666666667	275.2310946378616
33	115.825	276.50677093879307
34	124.77	277.24050407543166
35	135.845	276.9839543637859
36	145.535	276.33510232143624
37	155.00333333333333	275.133997636705
38	165.25666666666666	273.0307994632771
39	173.60833333333332	271.0464380825168
40	183.23666666666668	267.92192392975466
41	190.28166666666667	265.5293373569532
42	198.42	262.0655839034697
43	203.95833333333334	259.73590419993315
44	211.75166666666667	255.52633262325207
45	218.79166666666666	251.33619237432433
46	224.565	247.6893937474904
47	230.57333333333332	243.45917786949167
48	238.67	236.82901236968425
49	243.825	232.47876829580136
50	250.04833333333335	226.5902086672963
51	253.14166666666668	223.77694608073884
52	257.955	218.70187388695857
53	263.495	212.28089090086766
54	266.73833333333334	208.47046920500668
55	270.355	203.87831086622916
56	273.17	200.18287747290626
57	277.02666666666664	194.61862523635438
58	280.5883333333333	189.15138257637884
59	283.17833333333334	185.02370982450387
60	286.1333333333333	179.9788845639658
61	288.2783333333333	176.18426205885152
62	291.28833333333336	170.42422127509352
63	292.47833333333335	168.16455095299412
64	293.6816666666667	165.78053865644847
65	294.73	163.64390333892706
66	295.9583333333333	161.0047823220033
67	296.35833333333335	160.22519547152763
68	296.9316666666667	159.00197167715348
69	297.175	158.5519190728026
70	297.7583333333333	157.23522696019077
71	298.685	154.99003981439313
72	299.79	152.1830780124168
73	300.40166666666664	150.61799471031156
74	301.525	147.55721842164863
75	301.9866666666667	146.29788044336874
76	302.79	143.98454511972315
77	303.265	142.59312083103177
78	303.745	141.1450789377123
79	303.8933333333333	140.71078597210987
80	303.875	140.80214028321208
81	304.3616666666667	139.2478636480845
82	304.685	138.19500391958186
83	304.675	138.24689041108581
84	304.8333333333333	137.72311191501527
85	304.825	137.76711403064886
86	304.81666666666666	137.81140393870072
87	304.80833333333334	137.85598136178933
88	304.8	137.9008460210908
89	304.96	137.3377165967171
90	305.29	136.13687683112704
91	305.2866666666667	136.15543013613353
92	305.62	134.89995898195522
93	305.62	134.89995898195522
94	305.62	134.89995898195522
95	305.62	134.89995898195522
96	305.62	134.89995898195522
97	305.62	134.89995898195522
98	305.62	134.89995898195522
99	305.62	134.89995898195522
100	305.62	134.89995898195522
101	305.62	134.89995898195522
102	305.62	134.89995898195522
103	305.62	134.89995898195522
104	305.62	134.89995898195522
105	305.62	134.89995898195522
106	305.62	134.89995898195522
107	305.62	134.89995898195522
108	305.62	134.89995898195522
109	305.62	134.89995898195522
110	305.62	134.89995898195522
111	305.62	134.89995898195522
112	305.62	134.89995898195522
113	305.62	134.89995898195522
114	305.62	134.89995898195522
115	305.62	134.89995898195522
116	305.62	134.89995898195522
117	305.62	134.89995898195522
118	305.62	134.89995898195522
119	305.62	134.89995898195522
120	305.62	134.89995898195522
121	305.62	134.89995898195522
122	305.62	134.89995898195522
123	305.62	134.89995898195522
124	305.62	134.89995898195522
125	305.62	134.89995898195522
126	305.62	134.89995898195522
127	305.62	134.89995898195522
128	305.62	134.89995898195522
129	305.62	134.89995898195522
130	305.62	134.89995898195522
131	305.62	134.89995898195522
132	305.62	134.89995898195522
133	305.62	134.89995898195522
134	305.62	134.89995898195522
135	305.62	134.89995898195522
136	305.62	134.89995898195522
137	305.62	134.89995898195522
138	305.62	134.89995898195522
139	305.62	134.89995898195522
140	305.62	134.89995898195522
141	305.62	134.89995898195522
142	305.62	134.89995898195522
143	305.62	134.89995898195522
144	305.62	134.89995898195522
145	305.62	134.89995898195522
146	305.62	134.89995898195522
147	305.62	134.89995898195522
148	305.62	134.89995898195522
149	305.62	134.89995898195522
150	305.62	134.89995898195522
151	305.62	134.89995898195522
152	305.62	134.89995898195522
153	305.62	134.89995898195522
154	305.62	134.89995898195522
155	305.62	134.89995898195522
156	305.62	134.89995898195522
157	305.62	134.89995898195522
158	305.62	134.89995898195522
159	305.62	134.89995898195522
160	305.62	134.89995898195522
161	305.62	134.89995898195522
162	305.62	134.89995898195522
163	305.62	134.89995898195522
164	305.62	134.89995898195522
165	305.62	134.89995898195522
166	305.62	134.89995898195522
167	305.62	134.89995898195522
168	305.62	134.89995898195522
169	305.62	134.89995898195522
170	305.62	134.89995898195522
171	305.62	134.89995898195522
172	305.62	134.89995898195522
173	305.62	134.89995898195522
174	305.62	134.89995898195522
175	305.62	134.89995898195522
176	305.62	134.89995898195522
177	305.62	134.89995898195522
178	305.62	134.89995898195522
179	305.62	134.89995898195522
180	305.62	134.89995898195522
181	305.62	134.89995898195522
182	305.62	134.89995898195522
183	305.62	134.89995898195522
184	305.62	134.89995898195522
185	305.62	134.89995898195522
186	305.62	134.89995898195522
187	305.62	134.89995898195522
188	305.62	134.89995898195522
189	305.62	134.89995898195522
190	305.62	134.89995898195522
191	305.62	134.89995898195522
192	305.62	134.89995898195522
193	305.62	134.89995898195522
194	305.62	134.89995898195522
195	305.62	134.89995898195522
196	305.62	134.89995898195522
197	305.62	134.89995898195522
198	305.62	134.89995898195522
199	305.62	134.89995898195522
200	305.62	134.89995898195522
201	305.62	134.89995898195522
202	305.62	134.89995898195522
203	305.62	134.89995898195522
204	305.62	134.89995898195522
205	305.62	134.89995898195522
206	305.62	134.89995898195522
207	305.62	134.89995898195522
208	305.62	134.89995898195522
209	305.62	134.89995898195522
210	305.62	134.89995898195522
211	305.62	134.89995898195522
212	305.62	134.89995898195522
213	305.62	134.89995898195522
214	305.62	134.89995898195522
215	305.62	134.89995898195522
216	305.62	134.89995898195522
217	305.62	134.89995898195522
218	305.62	134.89995898195522
219	305.62	134.89995898195522
220	305.62	134.89995898195522
221	305.62	134.89995898195522
222	305.62	134.89995898195522
223	305.62	134.89995898195522
224	305.62	134.89995898195522
225	305.62	134.89995898195522
226	305.62	134.89995898195522
227	305.62	134.89995898195522
228	305.62	134.89995898195522
229	305.62	134.89995898195522
230	305.62	134.89995898195522
231	305.62	134.89995898195522
232	305.62	134.89995898195522
233	305.62	134.89995898195522
234	305.62	134.89995898195522
235	305.62	134.89995898195522
236	305.62	134.89995898195522
237	305.62	134.89995898195522
238	305.62	134.89995898195522
239	305.62	134.89995898195522
240	305.62	134.89995898195522
241	305.62	134.89995898195522
242	305.62	134.89995898195522
243	305.62	134.89995898195522
244	305.62	134.89995898195522
245	305.62	134.89995898195522
246	305.62	134.89995898195522
247	305.62	134.89995898195522
248	305.62	134.89995898195522
249	305.62	134.89995898195522
250	305.62	134.89995898195522
251	305.62	134.89995898195522
252	305.62	134.89995898195522
253	305.62	134.89995898195522
254	305.62	134.89995898195522
255	305.62	134.89995898195522
256	305.62	134.89995898195522
257	305.62	134.89995898195522
258	305.62	134.89995898195522
259	305.62	134.89995898195522
260	305.62	134.89995898195522
261	305.62	134.89995898195522
262	305.62	134.89995898195522
263	305.62	134.89995898195522
264	305.62	134.89995898195522
265	305.62	134.89995898195522
266	305.62	134.89995898195522
267	305.62	134.89995898195522
268	305.62	134.89995898195522
269	305.62	134.89995898195522
270	305.62	134.89995898195522
271	305.62	134.89995898195522
272	305.62	134.89995898195522
273	305.62	134.89995898195522
274	305.62	134.89995898195522
275	305.62	134.89995898195522
276	305.62	134.89995898195522
277	305.62	134.89995898195522
278	305.62	134.89995898195522
279	305.62	134.89995898195522
280	305.62	134.89995898195522
281	305.62	134.89995898195522
282	305.62	134.89995898195522
283	305.62	134.89995898195522
284	305.62	134.89995898195522
285	305.62	134.89995898195522
286	305.62	134.89995898195522
287	305.62	134.89995898195522
288	305.62	134.89995898195522
289	305.62	134.89995898195522
290	305.62	134.89995898195522
291	305.62	134.89995898195522
292	305.62	134.89995898195522
293	305.62	134.89995898195522
294	305.62	134.89995898195522
295	305.62	134.89995898195522
296	305.62	134.89995898195522
297	305.62	134.89995898195522
298	305.62	134.89995898195522
299	305.62	134.89995898195522
