# Supplementary material for: Task-Guided Inverse Reinforcement Learning Under Partial Information
Source: arXiv:2105.14073 source file (2021-12-16)
Supplement: Supplementary file 16 [file rock_mem10_trajsize10pomdp_irl_si.tex]

% $\mathrm{Guided \ policy, \ |n|=10}$
x	y	err
0	0.0	0.0
1	-0.09999999999999991	9.71445146547012e-17
2	-0.19999999999999982	1.942890293094024e-16
3	-0.4757666666666412	0.8303790774232093
4	-2.2771999999999855	2.215984392243475
5	-3.3412999999999373	3.4615898529432654
6	-4.0993999999999815	6.14087178718682
7	-2.634233333333317	14.954614608170091
8	5.134366666666787	30.50986696571357
9	24.06133333333282	43.54759340716277
10	35.53103333333293	46.69451973839067
11	39.126733333332815	47.37587317044583
12	43.135999999999605	47.797085796799365
13	46.4729999999997	47.840027428225135
14	50.453766666666624	47.61622509690236
15	53.737766666666744	47.087004615698966
16	56.6295333333333	46.525368719107355
17	58.58786666666665	46.037090547900085
18	61.61609999999997	45.146433791865945
19	63.577899999999985	44.441089038448524
20	65.34039999999995	43.798644512967705
21	66.6678666666666	43.226417163375984
22	68.19726666666651	42.558839025465936
23	69.29149999999977	42.000705443479944
24	70.8207666666664	41.205777977675844
25	72.08156666666635	40.464743298484166
26	73.84356666666628	39.36210705673132
27	75.03993333333287	38.548508989698945
28	76.53736666666613	37.47541621381799
29	77.23433333333276	36.92742442353048
30	78.63229999999939	35.81059610473828
31	79.16323333333268	35.35515820280788
32	80.16016666666603	34.47557932757934
33	80.72436666666603	33.946147787324975
34	81.38863333333268	33.30760224731825
35	82.05136666666593	32.651681602416055
36	83.18303333333253	31.450729119246684
37	83.74786666666586	30.806139357529656
38	84.47993333333247	29.953767553719292
39	84.84493333333242	29.519194450315666
40	85.51033333333237	28.6939146839341
41	85.70863333333232	28.425935143788664
42	86.47413333333229	27.406209349626433
43	86.80593333333226	26.919574503736342
44	87.27129999999892	26.258051583784123
45	87.70316666666558	25.60072264550793
46	88.2352666666656	24.78868686038491
47	88.50043333333224	24.348992240862028
48	89.0660333333323	23.404414888340344
49	89.43153333333228	22.74591184474471
50	89.86413333333232	21.96246768729655
51	90.0966666666656	21.51662540662192
52	90.46276666666563	20.79095100467718
53	90.52866666666564	20.662156991842647
54	90.89473333333235	19.91197844503533
55	91.02749999999902	19.63472061807831
56	91.32713333333237	18.957942146997297
57	91.46003333333233	18.662047743987827
58	91.55973333333236	18.436533620203505
59	91.65926666666569	18.201382570074742
60	91.82553333333239	17.811534129571402
61	91.92506666666571	17.56654486029873
62	92.15809999999905	16.984540060203916
63	92.2578333333324	16.72434907469404
64	92.39089999999908	16.346676538571042
65	92.49049999999907	16.07380497631681
66	92.52346666666573	15.986312144526128
67	92.68986666666571	15.530307916529706
68	92.88976666666574	14.943453815820309
69	92.92286666666571	14.847790984370397
70	92.95599999999905	14.740588771597082
71	93.02249999999906	14.543643184681583
72	93.15576666666573	14.137887398012756
73	93.15556666666572	14.13922047635183
74	93.1886666666657	14.037243730717107
75	93.25513333333237	13.819296182592648
76	93.38839999999904	13.38981573584951
77	93.4216666666657	13.248371367413045
78	93.4549666666657	13.137340496927916
79	93.45493333333236	13.137579013231033
80	93.48819999999904	13.025779596374626
81	93.48809999999905	13.02652147441253
82	93.52136666666573	12.903336266209944
83	93.58803333333239	12.662627168123144
84	93.5879333333324	12.663368735407165
85	93.58779999999906	12.664358300364151
86	93.58766666666571	12.665348839342194
87	93.68759999999907	12.311894502472004
88	93.72089999999905	12.191612137995982
89	93.75413333333239	12.070857588239454
90	93.75403333333239	12.0716606313668
91	93.75389999999908	12.072724276511392
92	93.8538333333324	11.676291590464501
93	93.88709999999908	11.549472582041576
94	93.88699999999909	11.550289072861558
95	93.92026666666575	11.421975424398122
96	93.95349999999907	11.292089314353326
97	93.95336666666573	11.293204829994862
98	93.98659999999909	11.161723004984312
99	94.01986666666575	11.027985853374332
100	94.05313333333241	10.892811246362815
101	94.05306666666574	10.893391755045252
102	94.05299999999907	10.893972844345182
103	94.08629999999907	10.756409979325511
104	94.08626666666575	10.756705725370852
105	94.0862333333324	10.757001773057159
106	94.08619999999908	10.757298122360202
107	94.08616666666576	10.757590745092108
108	94.08613333333241	10.757883669611168
109	94.08609999999908	10.758176895893483
110	94.11939999999908	10.619062590768882
111	94.1193333333324	10.619656282364126
112	94.11926666666574	10.620250568084018
113	94.15256666666573	10.478882259679455
114	94.18589999999907	10.335490208822566
115	94.18586666666573	10.335795095148208
116	94.1858333333324	10.336100294867263
117	94.21916666666573	10.190917654406112
118	94.21916666666573	10.190917654406112
119	94.21916666666573	10.190917654406112
120	94.21916666666573	10.190917654406112
121	94.21913333333241	10.191226974652613
122	94.21909999999909	10.191536612470912
123	94.21903333333242	10.19215585955966
124	94.25233333333242	10.04476519829552
125	94.25229999999908	10.045079792780829
126	94.28563333333241	9.895067639935077
127	94.28556666666574	9.895705213823168
128	94.28549999999908	9.896343419836198
129	94.35216666666575	9.589669892070702
130	94.35209999999908	9.590371330489134
131	94.35203333333241	9.59107341223538
132	94.35196666666576	9.591776137168646
133	94.41863333333245	9.229163710699293
134	94.41863333333245	9.229163710699293
135	94.41863333333245	9.229163710699293
136	94.41863333333245	9.229163710699293
137	94.41863333333245	9.229163710699293
138	94.41863333333245	9.229163710699293
139	94.41863333333245	9.229163710699293
140	94.41863333333245	9.229163710699293
141	94.41863333333245	9.229163710699293
142	94.41863333333245	9.229163710699293
143	94.41863333333245	9.229163710699293
144	94.41863333333245	9.229163710699293
145	94.41863333333245	9.229163710699293
146	94.41863333333245	9.229163710699293
147	94.41863333333245	9.229163710699293
148	94.41863333333245	9.229163710699293
149	94.41863333333245	9.229163710699293
150	94.41863333333245	9.229163710699293
151	94.41863333333245	9.229163710699293
152	94.41863333333245	9.229163710699293
153	94.41863333333245	9.229163710699293
154	94.41863333333245	9.229163710699293
155	94.41863333333245	9.229163710699293
156	94.41863333333245	9.229163710699293
157	94.41863333333245	9.229163710699293
158	94.41863333333245	9.229163710699293
159	94.41863333333245	9.229163710699293
160	94.41863333333245	9.229163710699293
161	94.41863333333245	9.229163710699293
162	94.41859999999912	9.22950634505089
163	94.41859999999912	9.22950634505089
164	94.41859999999912	9.22950634505089
165	94.41859999999912	9.22950634505089
166	94.41859999999912	9.22950634505089
167	94.41859999999912	9.22950634505089
168	94.41859999999912	9.22950634505089
169	94.41859999999912	9.22950634505089
170	94.41859999999912	9.22950634505089
171	94.4185666666658	9.229849327709582
172	94.41853333333245	9.23019265863704
173	94.41849999999913	9.23053633779392
174	94.45183333333246	9.06571140647866
175	94.45183333333246	9.06571140647866
176	94.45183333333246	9.06571140647866
177	94.45183333333246	9.06571140647866
178	94.45183333333246	9.06571140647866
179	94.45183333333246	9.06571140647866
180	94.45183333333246	9.06571140647866
181	94.45183333333246	9.06571140647866
182	94.45183333333246	9.06571140647866
183	94.45183333333246	9.06571140647866
184	94.45183333333246	9.06571140647866
185	94.45183333333246	9.06571140647866
186	94.45183333333246	9.06571140647866
187	94.45183333333246	9.06571140647866
188	94.45183333333246	9.06571140647866
189	94.45183333333246	9.06571140647866
190	94.45183333333246	9.06571140647866
191	94.45183333333246	9.06571140647866
192	94.45183333333246	9.06571140647866
193	94.45183333333246	9.06571140647866
194	94.45183333333246	9.06571140647866
195	94.45183333333246	9.06571140647866
196	94.45183333333246	9.06571140647866
197	94.45183333333246	9.06571140647866
198	94.45183333333246	9.06571140647866
199	94.45183333333246	9.06571140647866
200	94.45183333333246	9.06571140647866
201	94.45183333333246	9.06571140647866
202	94.45183333333246	9.06571140647866
203	94.45183333333246	9.06571140647866
204	94.45183333333246	9.06571140647866
205	94.45183333333246	9.06571140647866
206	94.45183333333246	9.06571140647866
207	94.45183333333246	9.06571140647866
208	94.45183333333246	9.06571140647866
209	94.45183333333246	9.06571140647866
210	94.45183333333246	9.06571140647866
211	94.45183333333246	9.06571140647866
212	94.45183333333246	9.06571140647866
213	94.45183333333246	9.06571140647866
214	94.45183333333246	9.06571140647866
215	94.45183333333246	9.06571140647866
216	94.45183333333246	9.06571140647866
217	94.45183333333246	9.06571140647866
218	94.45183333333246	9.06571140647866
219	94.45183333333246	9.06571140647866
220	94.45183333333246	9.06571140647866
221	94.45183333333246	9.06571140647866
222	94.45183333333246	9.06571140647866
223	94.45183333333246	9.06571140647866
224	94.45183333333246	9.06571140647866
225	94.45183333333246	9.06571140647866
226	94.45183333333246	9.06571140647866
227	94.45183333333246	9.06571140647866
228	94.45183333333246	9.06571140647866
229	94.45183333333246	9.06571140647866
230	94.45183333333246	9.06571140647866
231	94.45183333333246	9.06571140647866
232	94.45183333333246	9.06571140647866
233	94.45183333333246	9.06571140647866
234	94.45183333333246	9.06571140647866
235	94.45183333333246	9.06571140647866
236	94.45183333333246	9.06571140647866
237	94.45183333333246	9.06571140647866
238	94.45183333333246	9.06571140647866
239	94.45183333333246	9.06571140647866
240	94.45183333333246	9.06571140647866
241	94.45183333333246	9.06571140647866
242	94.45183333333246	9.06571140647866
243	94.45183333333246	9.06571140647866
244	94.45183333333246	9.06571140647866
245	94.45183333333246	9.06571140647866
246	94.45183333333246	9.06571140647866
247	94.45183333333246	9.06571140647866
248	94.45183333333246	9.06571140647866
249	94.45183333333246	9.06571140647866
250	94.45183333333246	9.06571140647866
251	94.45183333333246	9.06571140647866
252	94.45183333333246	9.06571140647866
253	94.45183333333246	9.06571140647866
254	94.45183333333246	9.06571140647866
255	94.45183333333246	9.06571140647866
256	94.45183333333246	9.06571140647866
257	94.45183333333246	9.06571140647866
258	94.45183333333246	9.06571140647866
259	94.45183333333246	9.06571140647866
260	94.45183333333246	9.06571140647866
261	94.45183333333246	9.06571140647866
262	94.45183333333246	9.06571140647866
263	94.45183333333246	9.06571140647866
264	94.45183333333246	9.06571140647866
265	94.45183333333246	9.06571140647866
266	94.45183333333246	9.06571140647866
267	94.45183333333246	9.06571140647866
268	94.45183333333246	9.06571140647866
269	94.45183333333246	9.06571140647866
270	94.45183333333246	9.06571140647866
271	94.45183333333246	9.06571140647866
272	94.45183333333246	9.06571140647866
273	94.45183333333246	9.06571140647866
274	94.45183333333246	9.06571140647866
275	94.45183333333246	9.06571140647866
276	94.45183333333246	9.06571140647866
277	94.45183333333246	9.06571140647866
278	94.45183333333246	9.06571140647866
279	94.45183333333246	9.06571140647866
280	94.45183333333246	9.06571140647866
281	94.45183333333246	9.06571140647866
282	94.45183333333246	9.06571140647866
283	94.45183333333246	9.06571140647866
284	94.45183333333246	9.06571140647866
285	94.45183333333246	9.06571140647866
286	94.45183333333246	9.06571140647866
287	94.45183333333246	9.06571140647866
288	94.45183333333246	9.06571140647866
289	94.45183333333246	9.06571140647866
290	94.45183333333246	9.06571140647866
291	94.45183333333246	9.06571140647866
292	94.45183333333246	9.06571140647866
293	94.45183333333246	9.06571140647866
294	94.45183333333246	9.06571140647866
295	94.45183333333246	9.06571140647866
296	94.45183333333246	9.06571140647866
297	94.45183333333246	9.06571140647866
298	94.45183333333246	9.06571140647866
299	94.45183333333246	9.06571140647866
300	94.45183333333246	9.06571140647866
301	94.45183333333246	9.06571140647866
302	94.45183333333246	9.06571140647866
303	94.45183333333246	9.06571140647866
304	94.45183333333246	9.06571140647866
305	94.45183333333246	9.06571140647866
306	94.45183333333246	9.06571140647866
307	94.45183333333246	9.06571140647866
308	94.45183333333246	9.06571140647866
309	94.45183333333246	9.06571140647866
310	94.45183333333246	9.06571140647866
311	94.45183333333246	9.06571140647866
