# Supplementary material for: Task-Guided Inverse Reinforcement Learning Under Partial Information
Source: arXiv:2105.14073 source file (2021-12-16)
Supplement: Supplementary file 17 [file rock_mem1_trajsize10mdp_irl_si.tex]

% $\mathrm{Guided \ policy, \ |n|=1}$
x	y	err
0	0.0	0.0
1	-0.10800000000000198	0.17870646322950048
2	-0.2160000000000041	0.25247574140895535
3	-0.2739666666666587	2.6162426490846706
4	-0.608333333333355	4.26746418327751
5	-0.6714333333333404	7.772556461393955
6	-0.5777666666666371	10.737576806658351
7	1.621600000000057	19.2126942438242
8	9.120566666666845	32.48441534560141
9	17.729233333332747	41.06063031760359
10	26.389266666666664	46.468090178052506
11	34.22169999999934	49.51041357576614
12	39.43393333333393	50.74743864008221
13	45.133199999999505	51.45471612100576
14	49.479366666667495	51.53016221203696
15	53.319833333333456	51.282138833179985
16	56.422166666665724	50.81756210837834
17	59.13789999999933	50.2074867616704
18	61.950966666666986	49.44368054395039
19	64.08116666666756	48.61301953837963
20	66.03823333333344	47.838399933653946
21	68.3044666666659	46.74366901926121
22	70.13909999999929	45.86336084345158
23	71.89823333333374	44.824470774480254
24	73.25753333333404	43.90098013236438
25	74.7384333333334	42.853444974846816
26	75.69343333333269	42.201912755374394
27	76.69086666666593	41.40290798863719
28	77.66146666666711	40.61825888910344
29	78.83723333333384	39.566430514754444
30	79.64473333333333	38.749953534538314
31	80.46229999999949	37.786325860598495
32	80.92173333333267	37.3671766081172
33	81.87673333333355	36.32697489922448
34	82.34040000000037	35.73772443567155
35	83.3421666666667	34.56028865580013
36	84.042033333333	33.63234935592335
37	84.70533333333286	32.70274654452668
38	85.3359333333335	31.83803148430432
39	85.84306666666687	31.192336002009018
40	86.52156666666664	30.141272891926068
41	86.89629999999975	29.540080618994036
42	87.53963333333299	28.3823071507389
43	88.02226666666674	27.506338133762583
44	88.37320000000008	26.825838820559948
45	88.62303333333328	26.351569203095956
46	88.90923333333318	25.881297843788495
47	89.22363333333313	25.24324103858735
48	89.34223333333341	25.07137437421852
49	89.76126666666674	24.20461580764204
50	89.98586666666662	23.586932404382107
51	90.24266666666651	22.97789356944814
52	90.46633333333313	22.47582019020051
53	90.65553333333341	21.828558115052534
54	90.77690000000004	21.518409089041246
55	90.93576666666667	21.19726108279607
56	91.09876666666659	20.587846458826732
57	91.4607666666665	19.321958943446223
58	91.62293333333334	18.60458708837398
59	91.78663333333328	18.050580544649737
60	91.81699999999991	17.867779688590254
61	91.91553333333322	17.362741873973196
62	92.04486666666648	16.999549611158002
63	92.07689999999992	16.83368576367034
64	92.17439999999996	16.422197111633185
65	92.2732333333333	16.10672199876668
66	92.43889999999995	15.592227875558105
67	92.46989999999991	15.476872551972523
68	92.53563333333331	15.235364133014826
69	92.63486666666665	14.869036876976653
70	92.70079999999999	14.614403147580198
71	92.70006666666663	14.619708387272576
72	92.69803333333329	14.642082711561914
73	92.72933333333336	14.5511529745546
74	92.72596666666668	14.584129584319495
75	92.72526666666667	14.589274882445443
76	92.75526666666664	14.488848318467415
77	92.75329999999997	14.503366819811163
78	92.75266666666668	14.508113117225948
79	92.75203333333334	14.512843594516143
80	92.75136666666666	14.517826219245874
81	92.78406666666665	14.396547715646562
82	92.85016666666665	13.925858201162683
83	92.84960000000004	13.930095710606805
84	92.88240000000002	13.792053155350047
85	92.88186666666668	13.796077383887885
86	92.88133333333333	13.80010428301985
87	92.88083333333333	13.803888678154768
88	92.88030000000005	13.807920742940704
89	92.8797666666667	13.811955471458559
90	92.87923333333336	13.815992861374696
91	92.87876666666666	13.819531557867183
92	92.91163333333333	13.69735015731956
93	92.91113333333337	13.701185205991822
94	92.9106666666667	13.704764362156068
95	92.9408666666667	13.602435440594993
96	92.97376666666668	13.467038345984694
97	93.00670000000001	13.31965509225619
98	93.0396666666667	13.180140359225653
99	93.03930000000003	13.183093422132199
100	93.03896666666668	13.18578824336595
101	93.0373	13.19950372968619
102	93.037	13.201918964049572
103	93.03663333333334	13.204887277023161
104	93.0696666666667	13.072242598558116
105	93.10270000000003	12.937898439983805
106	93.16913333333336	12.618811641707316
107	93.2022666666667	12.477920293952204
108	93.20213333333338	12.479073768335331
109	93.20060000000004	12.49256150568545
110	93.20043333333336	12.494014426071685
111	93.23363333333336	12.349968372384136
112	93.2334666666667	12.351451735817225
113	93.26666666666671	12.183221066514184
114	93.29990000000004	12.02306020348682
115	93.33316666666673	11.84879923475604
116	93.33310000000006	11.849411844335025
117	93.33303333333339	11.850024984455606
118	93.33296666666674	11.850638655035505
119	93.33290000000007	11.8512528559924
120	93.3328333333334	11.851867587243607
121	93.33276666666671	11.852482848706783
122	93.33270000000005	11.853098640299384
123	93.33266666666673	11.853418053690437
124	93.33260000000006	11.854034639733467
125	93.33120000000005	11.866762541934808
126	93.3311333333334	11.867390785210082
127	93.3644333333334	11.698406373471933
128	93.36440000000005	11.698731525540179
129	93.36436666666671	11.699056953399644
130	93.36433333333338	11.699382657027458
131	93.36430000000004	11.699708636400588
132	93.36426666666672	11.700034891495989
133	93.36423333333337	11.700361422290435
134	93.36423333333337	11.700361422290435
135	93.36423333333337	11.700361422290435
136	93.36423333333337	11.700361422290435
137	93.36420000000005	11.700688228761006
138	93.3641666666667	11.70101531088456
139	93.36413333333338	11.701342668638036
140	93.39746666666672	11.514745629650571
141	93.39746666666672	11.514745629650571
142	93.39746666666672	11.514745629650571
143	93.39746666666672	11.514745629650571
144	93.39746666666672	11.514745629650571
145	93.39746666666672	11.514745629650571
146	93.39746666666672	11.514745629650571
147	93.39746666666672	11.514745629650571
148	93.39746666666672	11.514745629650571
149	93.39746666666672	11.514745629650571
150	93.39746666666672	11.514745629650571
151	93.39746666666672	11.514745629650571
152	93.39746666666672	11.514745629650571
153	93.39746666666672	11.514745629650571
154	93.39746666666672	11.514745629650571
155	93.39746666666672	11.514745629650571
156	93.39746666666672	11.514745629650571
157	93.39746666666672	11.514745629650571
158	93.39746666666672	11.514745629650571
159	93.39746666666672	11.514745629650571
160	93.39746666666672	11.514745629650571
161	93.39746666666672	11.514745629650571
162	93.39746666666672	11.514745629650571
163	93.39746666666672	11.514745629650571
164	93.39746666666672	11.514745629650571
165	93.39746666666672	11.514745629650571
166	93.39746666666672	11.514745629650571
167	93.39746666666672	11.514745629650571
168	93.39746666666672	11.514745629650571
169	93.39746666666672	11.514745629650571
170	93.39746666666672	11.514745629650571
171	93.39746666666672	11.514745629650571
172	93.39746666666672	11.514745629650571
173	93.39746666666672	11.514745629650571
174	93.39746666666672	11.514745629650571
175	93.39746666666672	11.514745629650571
176	93.39746666666672	11.514745629650571
177	93.39746666666672	11.514745629650571
178	93.39746666666672	11.514745629650571
179	93.39746666666672	11.514745629650571
180	93.39746666666672	11.514745629650571
181	93.39746666666672	11.514745629650571
182	93.39746666666672	11.514745629650571
183	93.39746666666672	11.514745629650571
184	93.39746666666672	11.514745629650571
185	93.39746666666672	11.514745629650571
186	93.39746666666672	11.514745629650571
187	93.39746666666672	11.514745629650571
188	93.39746666666672	11.514745629650571
189	93.39746666666672	11.514745629650571
190	93.39746666666672	11.514745629650571
191	93.39746666666672	11.514745629650571
192	93.39746666666672	11.514745629650571
193	93.39746666666672	11.514745629650571
194	93.39746666666672	11.514745629650571
195	93.39746666666672	11.514745629650571
196	93.39746666666672	11.514745629650571
197	93.39746666666672	11.514745629650571
198	93.39746666666672	11.514745629650571
199	93.39746666666672	11.514745629650571
200	93.39746666666672	11.514745629650571
201	93.39746666666672	11.514745629650571
202	93.39746666666672	11.514745629650571
203	93.39746666666672	11.514745629650571
204	93.39746666666672	11.514745629650571
205	93.39746666666672	11.514745629650571
206	93.39746666666672	11.514745629650571
207	93.39746666666672	11.514745629650571
208	93.39746666666672	11.514745629650571
209	93.39746666666672	11.514745629650571
210	93.39746666666672	11.514745629650571
211	93.39746666666672	11.514745629650571
212	93.39746666666672	11.514745629650571
213	93.39746666666672	11.514745629650571
214	93.39746666666672	11.514745629650571
215	93.39746666666672	11.514745629650571
216	93.39746666666672	11.514745629650571
217	93.39746666666672	11.514745629650571
218	93.39746666666672	11.514745629650571
219	93.39746666666672	11.514745629650571
220	93.39746666666672	11.514745629650571
221	93.39746666666672	11.514745629650571
222	93.39746666666672	11.514745629650571
223	93.39746666666672	11.514745629650571
224	93.39746666666672	11.514745629650571
225	93.39746666666672	11.514745629650571
226	93.39746666666672	11.514745629650571
227	93.39746666666672	11.514745629650571
228	93.39746666666672	11.514745629650571
229	93.39746666666672	11.514745629650571
230	93.39746666666672	11.514745629650571
231	93.39746666666672	11.514745629650571
232	93.39746666666672	11.514745629650571
233	93.39746666666672	11.514745629650571
234	93.39746666666672	11.514745629650571
235	93.39746666666672	11.514745629650571
236	93.39746666666672	11.514745629650571
237	93.39746666666672	11.514745629650571
238	93.39746666666672	11.514745629650571
239	93.39746666666672	11.514745629650571
240	93.39746666666672	11.514745629650571
241	93.39746666666672	11.514745629650571
242	93.39746666666672	11.514745629650571
243	93.39746666666672	11.514745629650571
244	93.39746666666672	11.514745629650571
245	93.39746666666672	11.514745629650571
246	93.39746666666672	11.514745629650571
247	93.39746666666672	11.514745629650571
248	93.39746666666672	11.514745629650571
249	93.39746666666672	11.514745629650571
250	93.39746666666672	11.514745629650571
251	93.39746666666672	11.514745629650571
252	93.39746666666672	11.514745629650571
253	93.39746666666672	11.514745629650571
254	93.39746666666672	11.514745629650571
255	93.39746666666672	11.514745629650571
256	93.39746666666672	11.514745629650571
257	93.39746666666672	11.514745629650571
258	93.39746666666672	11.514745629650571
259	93.39746666666672	11.514745629650571
260	93.39746666666672	11.514745629650571
261	93.39746666666672	11.514745629650571
262	93.39746666666672	11.514745629650571
263	93.39746666666672	11.514745629650571
264	93.39746666666672	11.514745629650571
265	93.39746666666672	11.514745629650571
266	93.39746666666672	11.514745629650571
267	93.39746666666672	11.514745629650571
268	93.39746666666672	11.514745629650571
269	93.39746666666672	11.514745629650571
270	93.39746666666672	11.514745629650571
271	93.39746666666672	11.514745629650571
272	93.39746666666672	11.514745629650571
273	93.39746666666672	11.514745629650571
274	93.39746666666672	11.514745629650571
275	93.39746666666672	11.514745629650571
276	93.39746666666672	11.514745629650571
277	93.39746666666672	11.514745629650571
278	93.39746666666672	11.514745629650571
279	93.39746666666672	11.514745629650571
280	93.39746666666672	11.514745629650571
281	93.39746666666672	11.514745629650571
282	93.39746666666672	11.514745629650571
283	93.39746666666672	11.514745629650571
284	93.39746666666672	11.514745629650571
285	93.39746666666672	11.514745629650571
286	93.39746666666672	11.514745629650571
287	93.39746666666672	11.514745629650571
288	93.39746666666672	11.514745629650571
289	93.39746666666672	11.514745629650571
290	93.39746666666672	11.514745629650571
291	93.39746666666672	11.514745629650571
292	93.39746666666672	11.514745629650571
293	93.39746666666672	11.514745629650571
294	93.39746666666672	11.514745629650571
295	93.39746666666672	11.514745629650571
296	93.39746666666672	11.514745629650571
297	93.39746666666672	11.514745629650571
298	93.39746666666672	11.514745629650571
299	93.39746666666672	11.514745629650571
300	93.39746666666672	11.514745629650571
301	93.39746666666672	11.514745629650571
302	93.39746666666672	11.514745629650571
303	93.39746666666672	11.514745629650571
304	93.39746666666672	11.514745629650571
305	93.39746666666672	11.514745629650571
306	93.39746666666672	11.514745629650571
307	93.39746666666672	11.514745629650571
308	93.39746666666672	11.514745629650571
309	93.39746666666672	11.514745629650571
310	93.39746666666672	11.514745629650571
311	93.39746666666672	11.514745629650571
